# Supplementary material for: Data Valuation Without Training of a Model
Source: arXiv:2301.00930 source file (2023-03-07)
Supplement: Supplementary file 1 [file addi_noise.tex]

\begin{figure*}[!tb]
\centering
	\includegraphics[width=0.8\linewidth]{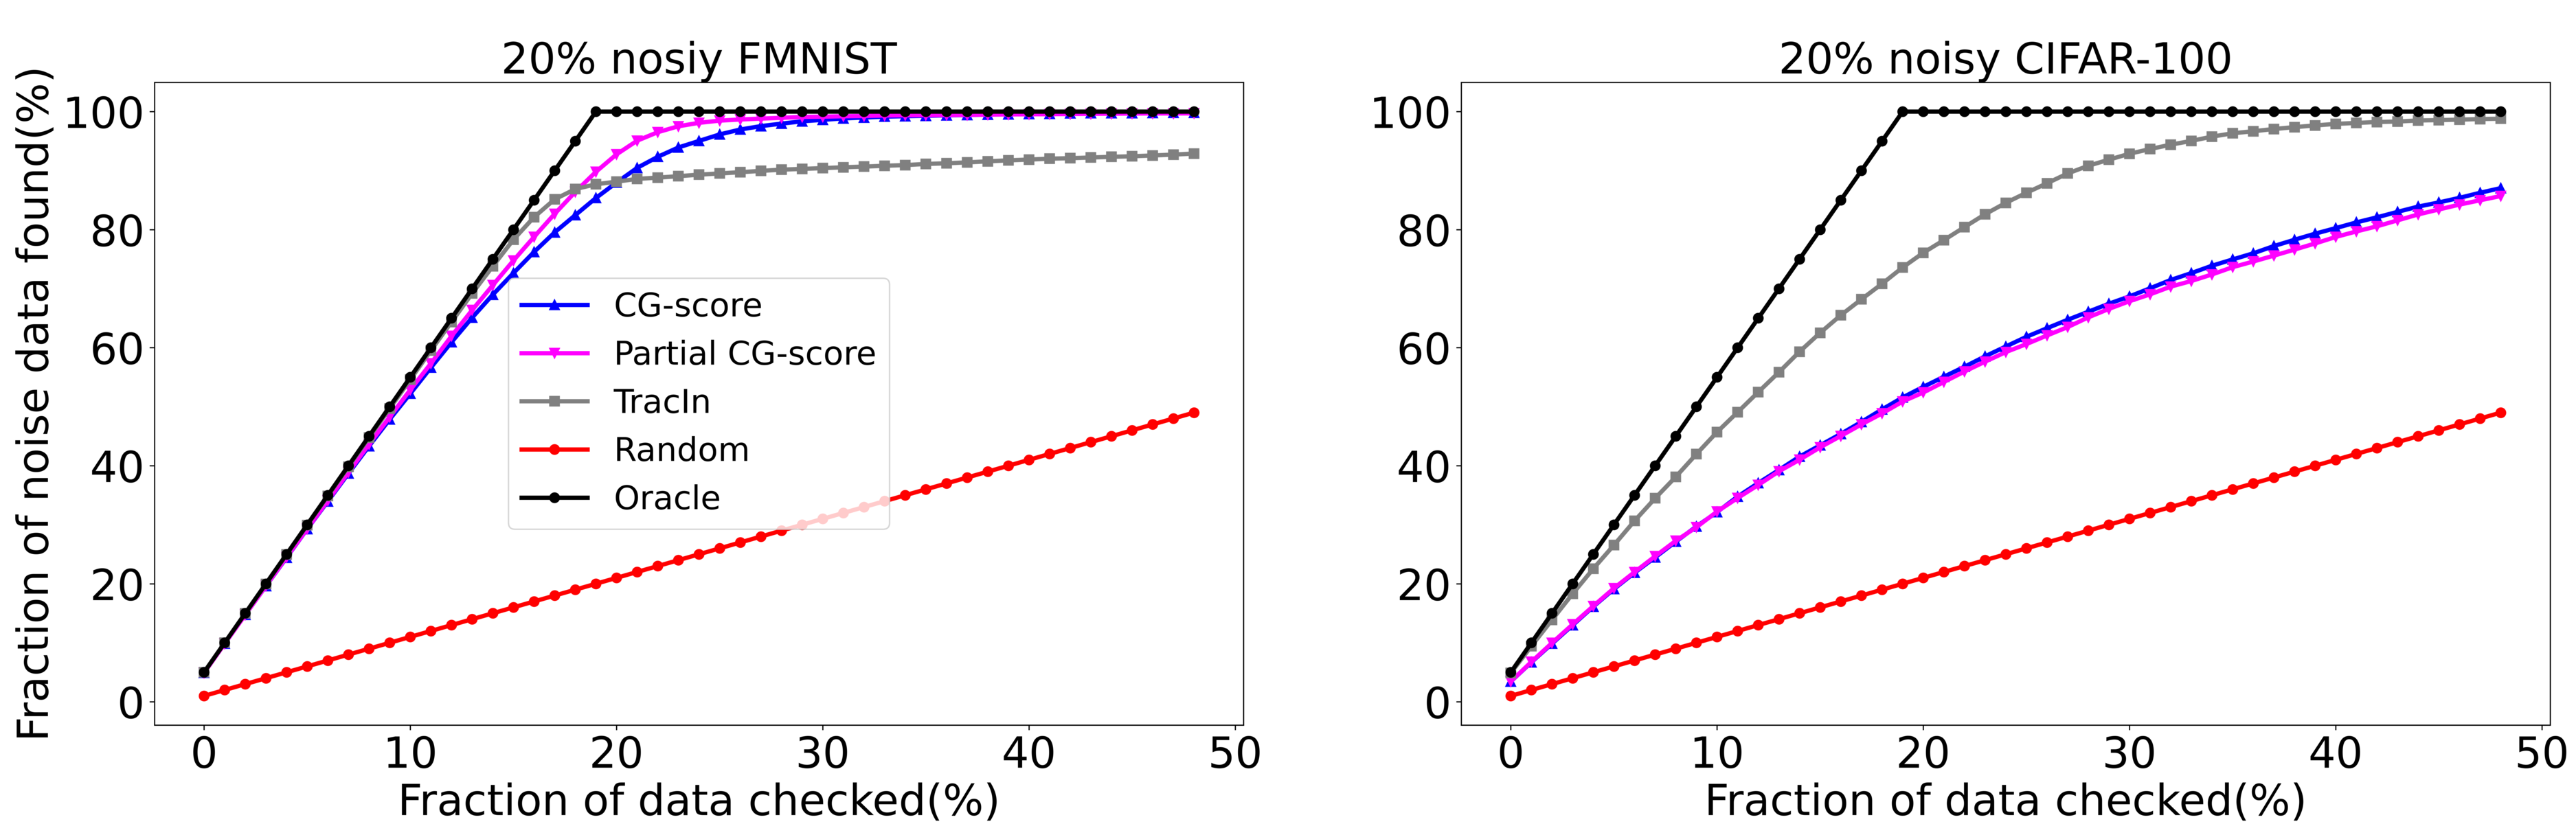} 
    \caption{Fraction of label noise (y-axis) included in the examined portion (x-axis) for 20\% label noise for oracle, Partial CG-score (ours), CG-score (ours), TracIn and random baseline.}
    \label{fig:addi_noise}
\end{figure*}
