# Supplementary material for: Data Valuation Without Training of a Model
Source: arXiv:2301.00930 source file (2023-03-07)
Supplement: Supplementary file 8 [file tiny_pruning.tex]

\begin{figure*}[!tb]
\centering
    \begin{tabular}{cc}
	    \includegraphics[ width=0.4\linewidth]{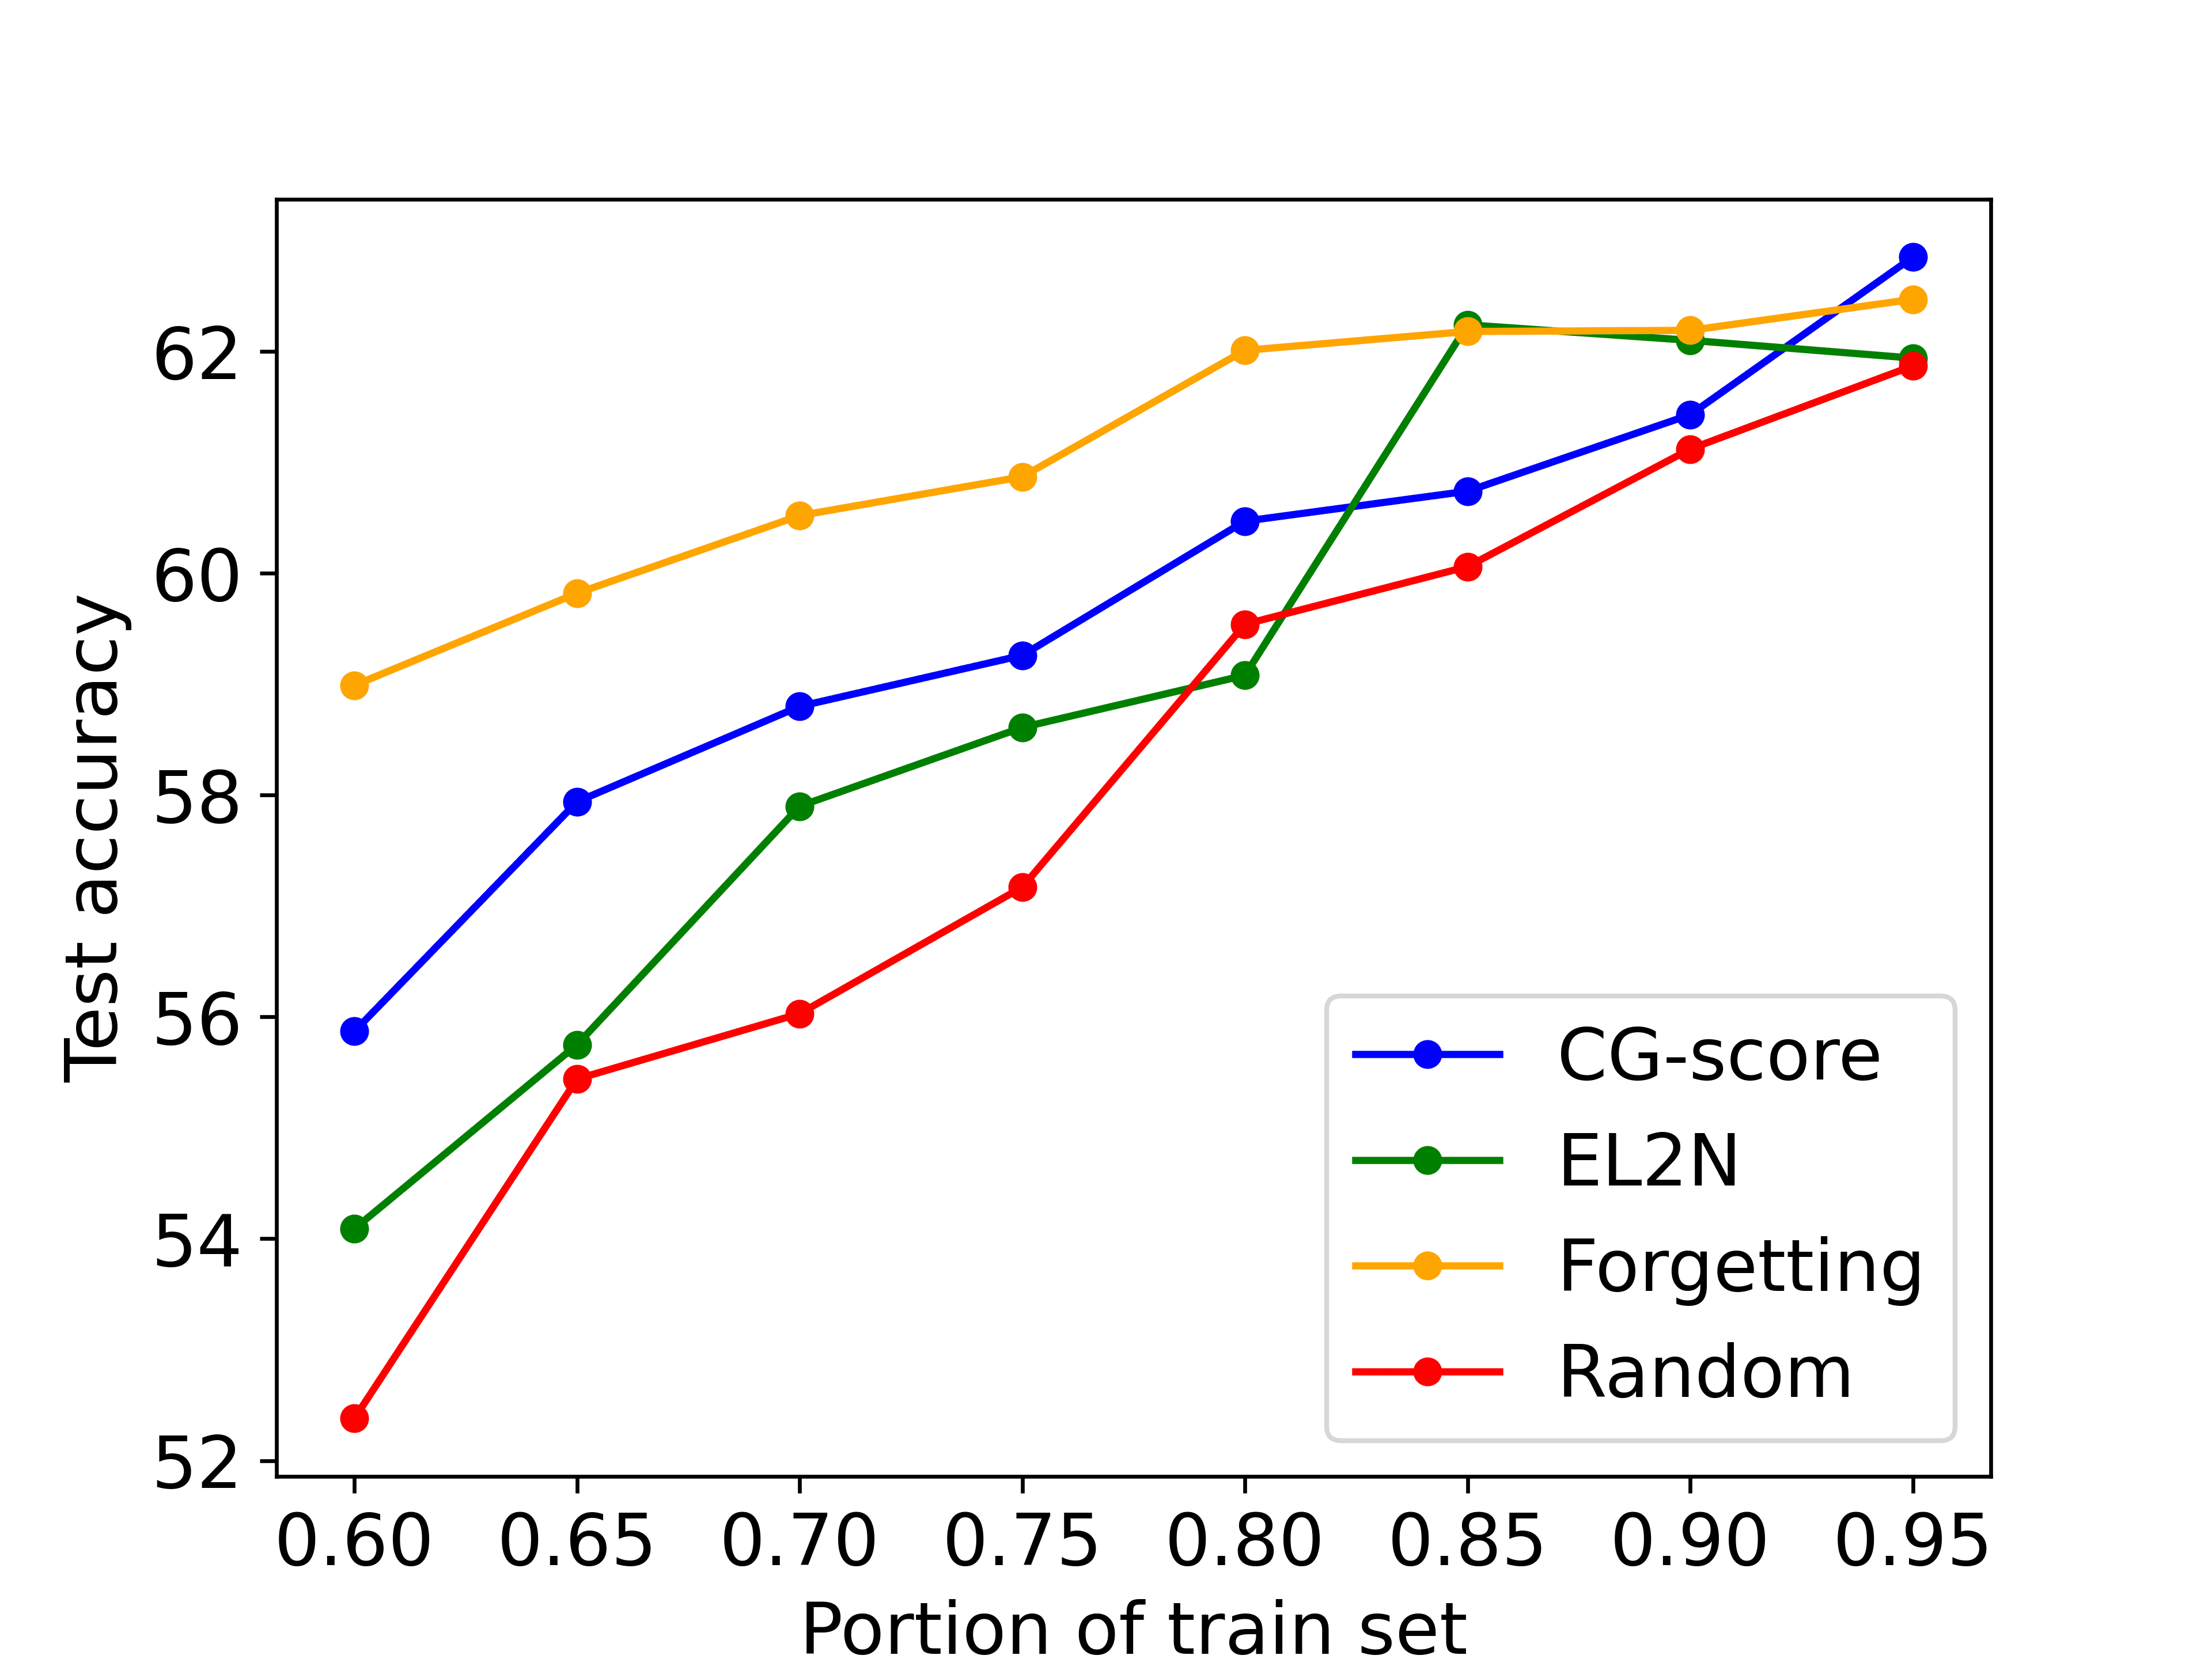} & 
	    \includegraphics[ width=0.4\linewidth]{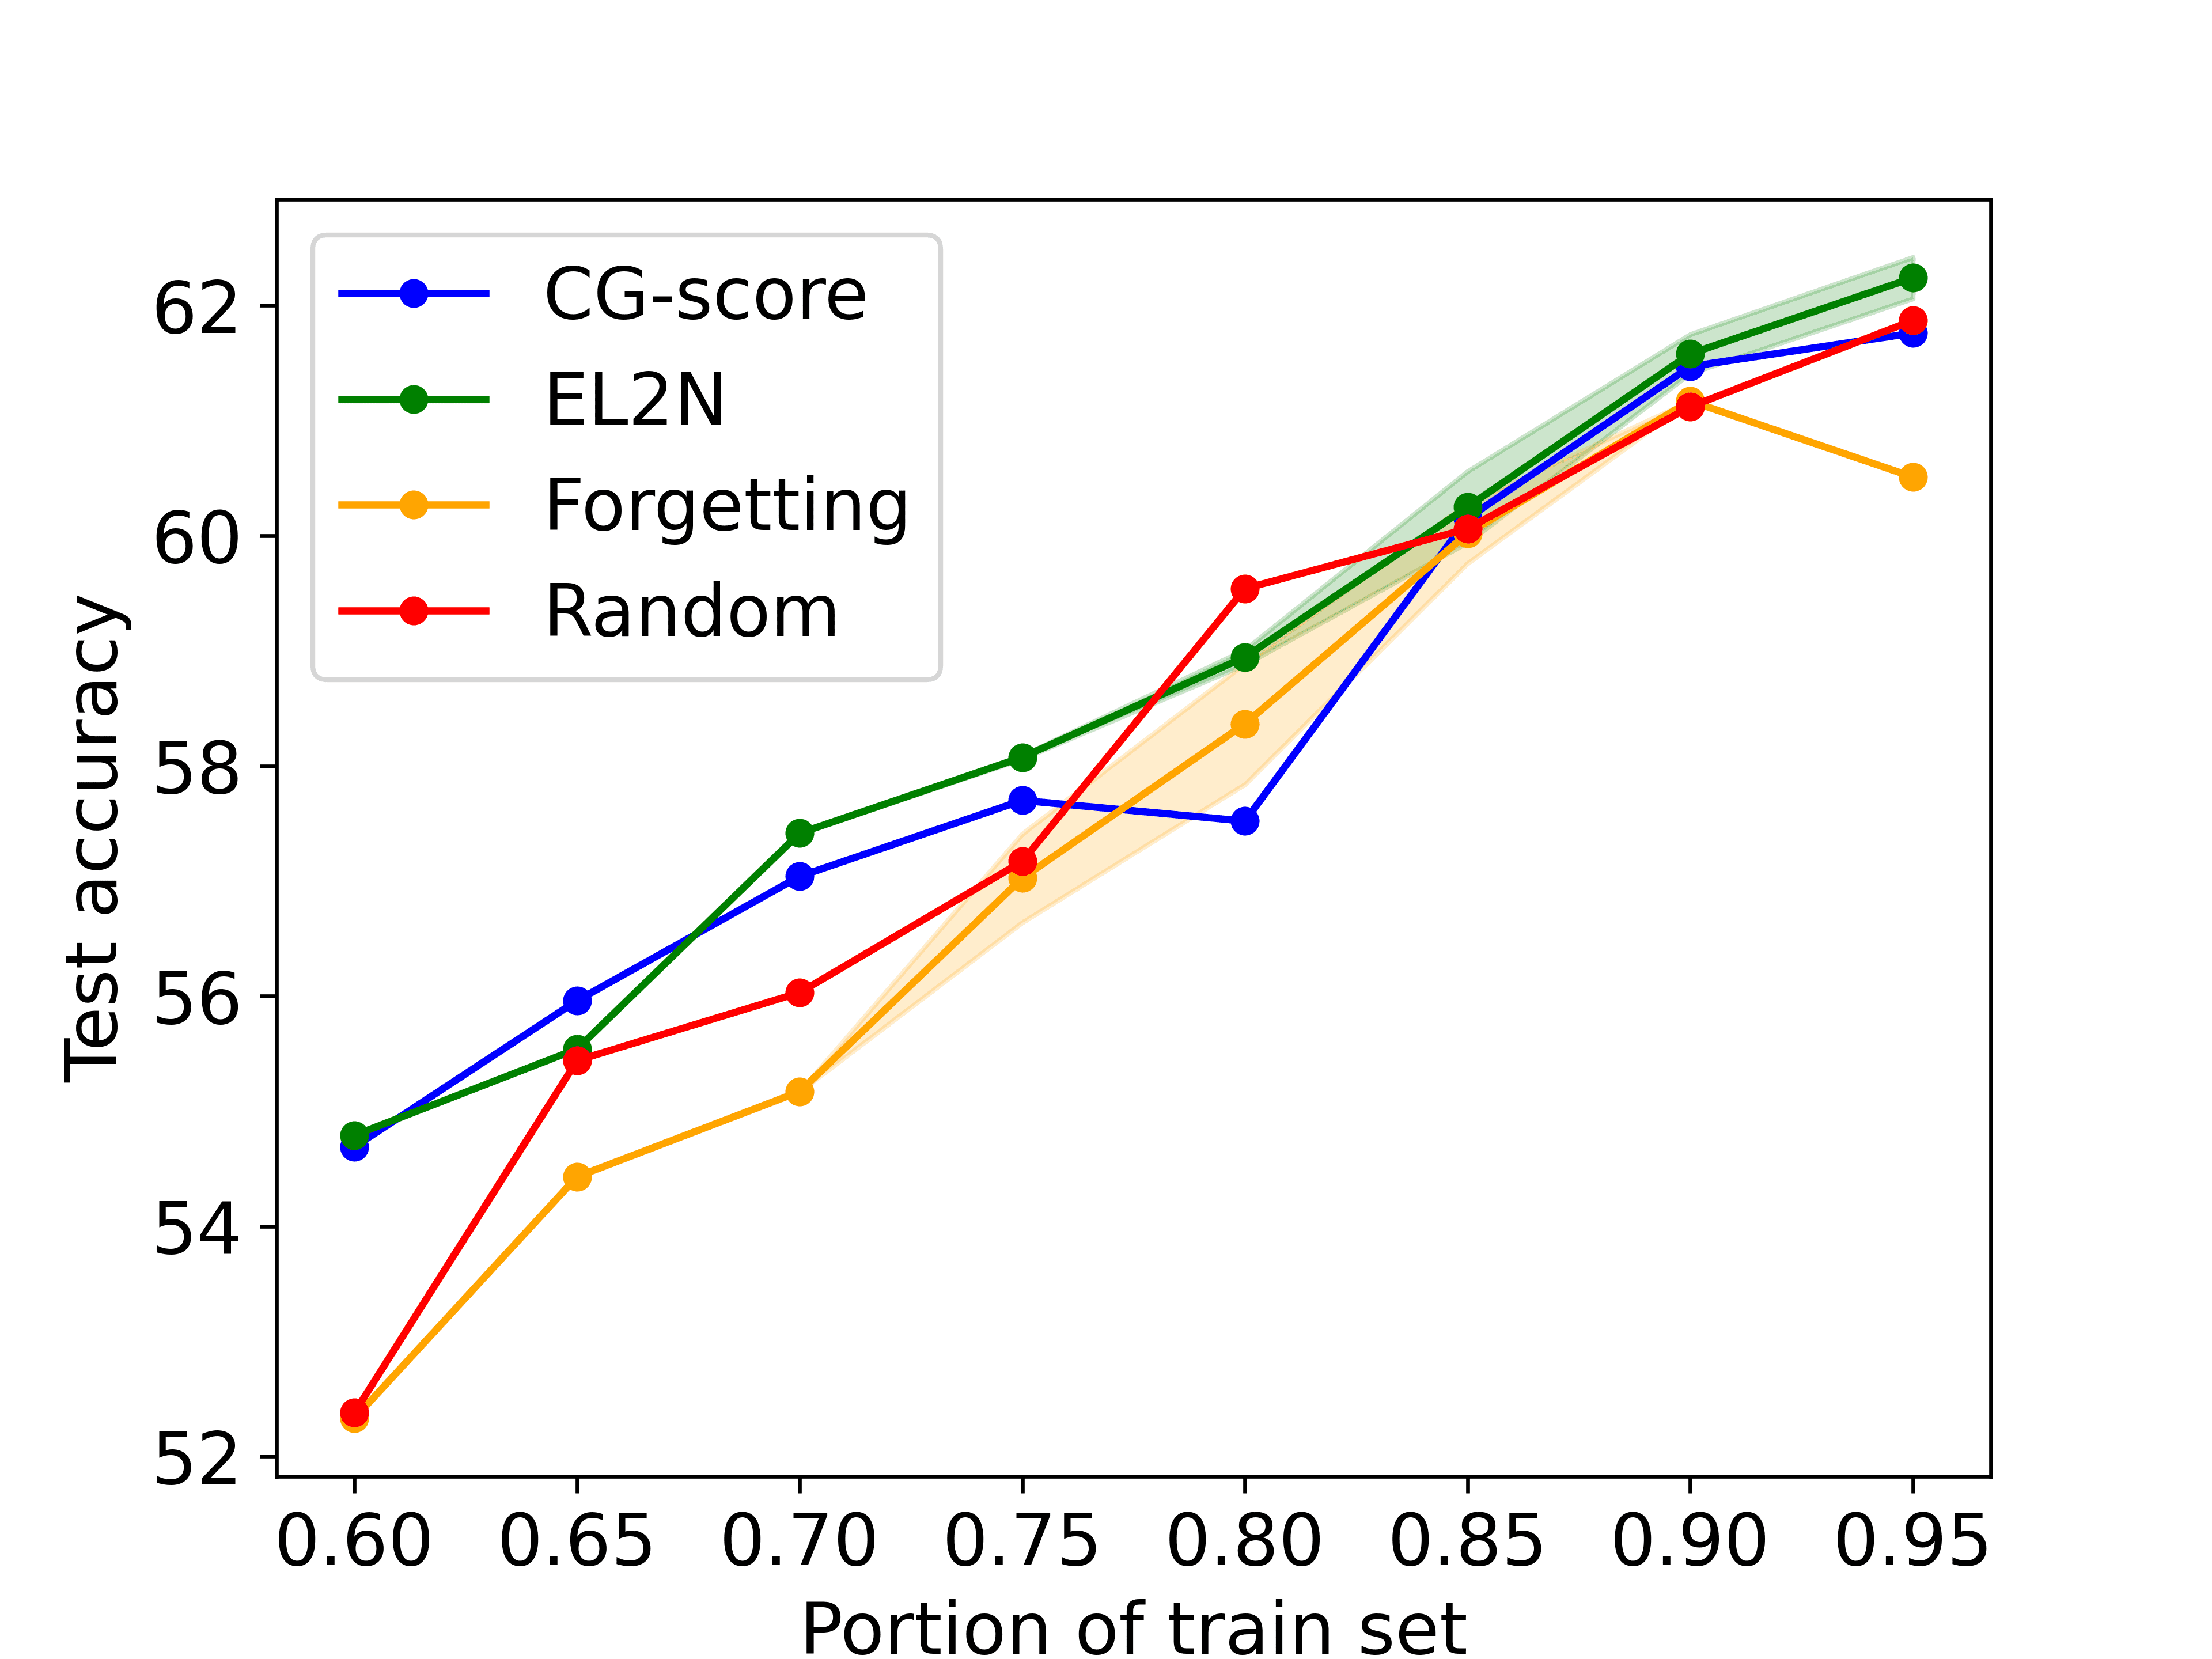}
    \end{tabular}
    \caption{
    Pruning experiments with three datasets FMNIST (left), CIFAR-10 (middle) and CIFAR-100 (right). 
    The test accuracy of the model trained with different portions ($x$-axis) of subset data when the low-scoring examples are removed first (top row) / the high-scoring examples are removed first (bottom row). Only CG-Score does not require any training of the model to calculate the score for examples, but it achieves competitive performances compared to other state-of-the-art data valuation scores and significantly outperforms the performance of random baseline. When low-scoring examples are removed first, CG-score maintains the test accuracy up to significant removing portions; when high-scoring examples are removed first, the test accuracy drops most rapidly for CG-score since the examples with high CG-score are essential in generalization of the model. 
 %   Final test accuracy according to the amount of training data for each score. The first row is the final test accuracy when pruning data with low values, and the second is the final test accuracy when pruning data with high values(labeled to the left). Each column is arranged according to which training data is used(labeled above).
    }
\end{figure*}
