# Supplementary material for: Data Valuation Without Training of a Model
Source: arXiv:2301.00930 source file (2023-03-07)
Supplement: Supplementary file 9 [file CIFAR10_noise_exp.tex]

\begin{figure*}[!tb]
\centering
	\subfloat[Noise rate 5\%]{\includegraphics[width=0.25\linewidth]{fig/noise_exp/CIFAR10_noise_5_detect.png}}
    \subfloat[Noise rate 10\%]{\includegraphics[width=0.25\linewidth]{fig/noise_exp/CIFAR10_noise_10_detect.png}}
    \subfloat[Noise rate 20\%]{\includegraphics[width=0.25\linewidth]{fig/noise_exp/CIFAR10_noise_20_detect.png}}
    \subfloat[Noise rate 30\%]{\includegraphics[width=0.25\linewidth]{fig/noise_exp/CIFAR10_noise_30_detect.png}}
    \caption{Noise detectability of oracle score(green) $CG$ score(blue), subterm score(red) and random(black) at CIFAR10 dataset. x-axis is fraction of checked data among whole data and y-axis is fraction of detected noisy data.}
    \label{fig:CIFAR10_noise_exp}
\end{figure*}
