# Supplementary material for: Data Valuation Without Training of a Model
Source: arXiv:2301.00930 source file (2023-03-07)
Supplement: Supplementary file 11 [file FMNIST_noise_exp.tex]

\begin{figure*}[!tb]
\centering
    \subfloat[Noise rate 20\%]{\includegraphics[width=0.25\linewidth]{fig/noise_exp/FMNIST_noise_20_detect.png}}
    \subfloat[Noise rate 20\%]{\includegraphics[width=0.25\linewidth]{fig/score_distribution/distribution_FMNIST_noisy.png}}
    \caption{Noise detectability of oracle score(green) $CG$ score(blue), subterm score(red) and random(black) at FMNIST dataset. x-axis is fraction of checked data among whole data and y-axis is fraction of detected noisy data.}
    \label{fig:FMNIST_noise_exp}
\end{figure*}
